# Supplementary material for: Multimer Embedding for Molecular Crystals Utilizing up to Tetramer Interactions
Source: arXiv:2512.16877 ancillary file (2025-12-18)
Supplement: Supplementary file 1 [file Supplementary_Material.pdf]

# Supplementary Material for:

# Multimer Embedding for Molecular Crystals Utilizing up to Tetramer Interactions

Alexander List[a], A. Daniel Boese*[a], and Johannes Hoja*[a]

[a] Department of Chemistry, University of Graz, Heinrichstraße 28/IV, 8010 Graz, Austria

* Correspondence to: adrian_daniel.boese@uni-graz.at, johannes.hoja@uni-graz.at

## Contents

**1 Number of Dimers, Trimers, and Tetramers** **2**

**2 Lattice Energies** **6**

**3 Unit-Cell Volumes** **16**

**4 Phonon Densities of States** **17**

# 1 Number of Dimers, Trimers, and Tetramers

**Table S1:** Number of identified unique dimers for a given cutoff distance for the X23 set evaluated on top of PBE0+MBD/light optimized structures; $Z$ lists the number of molecules within the unit cell and $n$ is the number of atoms per molecule.

| | $n$ | $Z$ | 3 Å | 4 Å | 5 Å | 6 Å | 7 Å | 8 Å |
|---|---|---|---|---|---|---|---|---|
| 1,4-Cyclohexanedione | 16 | 2 | 6 | 8 | 9 | 14 | 20 | 28 |
| Acetic acid | 8 | 4 | 5 | 8 | 11 | 17 | 26 | 35 |
| Adamantane | 26 | 2 | 2 | 2 | 4 | 5 | 8 | 8 |
| Ammonia | 4 | 4 | 2 | 3 | 5 | 8 | 13 | 16 |
| Anthracene | 24 | 2 | 4 | 5 | 6 | 11 | 13 | 15 |
| Benzene | 12 | 4 | 3 | 3 | 6 | 9 | 12 | 17 |
| Carbon dioxide | 3 | 4 | 0 | 1 | 2 | 3 | 5 | 9 |
| Cyanamide | 5 | 8 | 5 | 9 | 11 | 24 | 31 | 40 |
| Cytosine | 13 | 4 | 4 | 7 | 10 | 17 | 21 | 28 |
| Ethyl carbamate | 13 | 2 | 10 | 12 | 15 | 25 | 30 | 40 |
| Formamide | 6 | 4 | 6 | 9 | 15 | 23 | 36 | 46 |
| Hexamine | 22 | 2 | 3 | 3 | 2 | 4 | 8 | 8 |
| Imidazole | 9 | 4 | 6 | 10 | 12 | 21 | 29 | 36 |
| Naphthalene | 18 | 2 | 4 | 5 | 6 | 12 | 13 | 16 |
| Oxalic acid $\alpha$ | 8 | 4 | 3 | 5 | 7 | 11 | 16 | 21 |
| Oxalic acid $\beta$ | 8 | 2 | 3 | 5 | 7 | 14 | 19 | 25 |
| Pyrazine | 10 | 2 | 3 | 4 | 4 | 8 | 10 | 16 |
| Pyrazole | 9 | 8 | 11 | 13 | 20 | 36 | 47 | 61 |
| s-Triazine | 9 | 6 | 9 | 11 | 14 | 23 | 30 | 45 |
| s-Trioxane | 12 | 6 | 4 | 4 | 5 | 7 | 11 | 14 |
| Succinic acid | 14 | 2 | 4 | 5 | 7 | 11 | 18 | 23 |
| Uracil | 12 | 4 | 5 | 10 | 11 | 19 | 26 | 37 |
| Urea | 8 | 2 | 3 | 5 | 5 | 9 | 12 | 14 |

**Table S2:** Number of identified unique trimers for each trimer type for a given cutoff distance for the X23 set evaluated on top of PBE0+MBD/light optimized structures; $Z$ lists the number of molecules within the unit cell and $n$ is the number of atoms per molecule.

| | | | Closed | | | | Open | | | |
|---|---|---|---|---|---|---|---|---|---|---|
| | $n$ | $Z$ | 3 Å | 4 Å | 5 Å | 6 Å | 3 Å | 4 Å | 5 Å | 6 Å |
| 1,4-Cyclohexanedione | 16 | 2 | 8 | 16 | 20 | 51 | 43 | 73 | 94 | 225 |
| Acetic acid | 8 | 4 | 4 | 16 | 32 | 77 | 33 | 73 | 136 | 331 |
| Adamantane | 26 | 2 | 2 | 2 | 6 | 12 | 12 | 12 | 26 | 52 |
| Ammonia | 4 | 4 | 7 | 11 | 22 | 65 | 14 | 31 | 89 | 211 |
| Anthracene | 24 | 2 | 4 | 6 | 7 | 30 | 24 | 31 | 43 | 136 |
| Benzene | 12 | 4 | 4 | 4 | 10 | 27 | 26 | 26 | 56 | 126 |
| Carbon dioxide | 3 | 4 | 0 | 5 | 5 | 15 | 0 | 8 | 17 | 52 |
| Cyanamide | 5 | 8 | 3 | 14 | 20 | 134 | 37 | 67 | 98 | 525 |
| Cytosine | 13 | 4 | 2 | 12 | 25 | 79 | 22 | 55 | 115 | 324 |
| Ethyl carbamate | 13 | 2 | 10 | 14 | 23 | 83 | 50 | 65 | 104 | 349 |
| Formamide | 6 | 4 | 3 | 12 | 32 | 92 | 27 | 55 | 161 | 397 |
| Hexamine | 22 | 2 | 1 | 1 | 1 | 21 | 7 | 7 | 8 | 16 |
| Imidazole | 9 | 4 | 3 | 14 | 19 | 71 | 36 | 63 | 97 | 316 |
| Naphthalene | 18 | 2 | 4 | 6 | 7 | 39 | 24 | 31 | 43 | 173 |
| Oxalic acid $\alpha$ | 8 | 4 | 4 | 8 | 19 | 40 | 24 | 42 | 98 | 181 |
| Oxalic acid $\beta$ | 8 | 2 | 2 | 6 | 12 | 44 | 20 | 32 | 65 | 194 |
| Pyrazine | 10 | 2 | 2 | 4 | 4 | 21 | 17 | 20 | 20 | 102 |
| Pyrazole | 9 | 8 | 12 | 20 | 50 | 175 | 74 | 96 | 234 | 739 |
| s-Triazine | 9 | 6 | 12 | 17 | 35 | 81 | 62 | 68 | 133 | 384 |
| s-Trioxane | 12 | 6 | 4 | 4 | 8 | 29 | 20 | 20 | 41 | 98 |
| Succinic acid | 14 | 2 | 2 | 6 | 14 | 34 | 19 | 31 | 79 | 154 |
| Uracil | 12 | 4 | 3 | 17 | 19 | 60 | 23 | 73 | 83 | 267 |
| Urea | 8 | 2 | 2 | 7 | 7 | 32 | 15 | 27 | 27 | 120 |

**Table S3:** Number of identified unique tetramers for each tetramer type for a given cutoff distance for the X23 set evaluated on top of PBE0+MBD/light optimized structures; $Z$ lists the number of molecules within the unit cell and $n$ is the number of atoms per molecule.

| | | | Closed | | | | Diamond | | Paw | | Ring | | Claw | | Open | |
|---|---|---|---|---|---|---|---|---|---|---|---|---|---|---|---|---|
| | $n$ | $Z$ | 3 Å | 4 Å | 5 Å | 6 Å | 3 Å | 4 Å | 3 Å | 4 Å | 3 Å | 4 Å | 3 Å | 4 Å | 3 Å | 4 Å |
| 1,4-Cyclohexanedione | 16 | 2 | 2 | 11 | 16 | 74 | 24 | 62 | 120 | 292 | 3 | 5 | 44 | 100 | 278 | 632 |
| Acetic acid | 8 | 4 | 1 | 11 | 38 | 151 | 8 | 61 | 52 | 296 | 7 | 3 | 48 | 98 | 201 | 651 |
| Adamantane | 26 | 2 | 3 | 3 | 7 | 20 | 6 | 6 | 30 | 30 | 2 | 3 | 11 | 11 | 74 | 74 |
| Ammonia | 4 | 4 | 4 | 8 | 30 | 197 | 8 | 28 | 40 | 140 | 1 | 3 | 21 | 64 | 94 | 319 |
| Anthracene | 24 | 2 | 1 | 3 | 4 | 51 | 14 | 24 | 60 | 100 | 3 | 1 | 22 | 30 | 148 | 227 |
| Benzene | 12 | 4 | 1 | 1 | 10 | 40 | 12 | 12 | 60 | 60 | 3 | 3 | 22 | 22 | 142 | 142 |
| Carbon dioxide | 3 | 4 | 0 | 5 | 5 | 21 | 0 | 4 | 0 | 20 | 0 | 1 | 0 | 19 | 0 | 47 |
| Cyanamide | 5 | 8 | 0 | 9 | 18 | 366 | 5 | 51 | 52 | 250 | 10 | 2 | 58 | 74 | 232 | 549 |
| Cytosine | 13 | 4 | 0 | 6 | 24 | 163 | 2 | 41 | 28 | 196 | 3 | 2 | 24 | 62 | 110 | 429 |
| Ethyl carbamate | 13 | 2 | 4 | 9 | 22 | 183 | 40 | 62 | 154 | 240 | 5 | 5 | 52 | 79 | 375 | 568 |
| Formamide | 6 | 4 | 0 | 6 | 35 | 207 | 7 | 46 | 41 | 196 | 4 | 3 | 32 | 62 | 159 | 445 |
| Hexamine | 22 | 2 | 0 | 4 | 2 | 38 | 0 | 4 | 3 | 11 | 0 | 2 | 0 | 24 | 3 | 28 |
| Imidazole | 9 | 4 | 0 | 9 | 15 | 133 | 7 | 54 | 50 | 248 | 11 | 2 | 59 | 75 | 235 | 555 |
| Naphthalene | 18 | 2 | 1 | 3 | 4 | 78 | 14 | 24 | 60 | 100 | 3 | 1 | 22 | 30 | 148 | 227 |
| Oxalic acid $\alpha$ | 8 | 4 | 1 | 6 | 22 | 75 | 12 | 32 | 60 | 146 | 3 | 3 | 22 | 50 | 141 | 334 |
| Oxalic acid $\beta$ | 8 | 2 | 0 | 3 | 11 | 98 | 6 | 25 | 28 | 96 | 5 | 2 | 22 | 32 | 102 | 225 |
| Pyrazine | 10 | 2 | 0 | 2 | 2 | 37 | 7 | 15 | 26 | 53 | 5 | 1 | 23 | 19 | 98 | 126 |
| Pyrazole | 9 | 8 | 2 | 8 | 49 | 377 | 31 | 64 | 176 | 308 | 8 | 4 | 84 | 104 | 470 | 700 |
| s-Triazine | 9 | 6 | 0 | 6 | 24 | 107 | 30 | 59 | 96 | 192 | 17 | 5 | 82 | 64 | 379 | 471 |
| s-Trioxane | 12 | 6 | 2 | 2 | 7 | 55 | 14 | 14 | 64 | 64 | 1 | 1 | 32 | 32 | 144 | 144 |
| Succinic acid | 14 | 2 | 0 | 3 | 14 | 62 | 7 | 25 | 28 | 96 | 3 | 2 | 22 | 32 | 108 | 225 |
| Uracil | 12 | 4 | 0 | 11 | 14 | 95 | 3 | 68 | 28 | 292 | 4 | 7 | 24 | 100 | 116 | 663 |
| Urea | 8 | 2 | 0 | 6 | 6 | 67 | 5 | 20 | 20 | 91 | 3 | 2 | 18 | 34 | 63 | 192 |

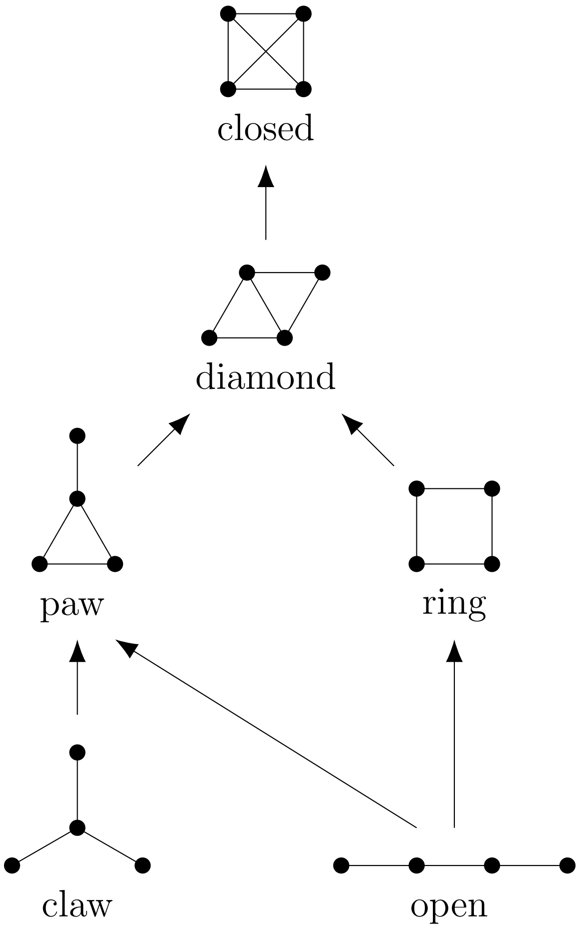


**Figure S1:** Tetramer types to illustrate the labeling scheme of ME4 calculations. By adding edges one after another to the tetramer types with the lowest number of edges, an order of the tetramer types arises, which is indicated by arrows. Therefore, to label the calculations that use only certain tetramer types, we use the initials of the included tetramer type(s) with the lowest number of edges in their respective path, and higher-number of edges tetramer types along this path are included as well. This yields the following possibilities of including tetramer types: No additional label for only closed tetramers; 'd' for diamond and closed; 'p' for paw, diamond, and closed; 'r' for ring, diamond, and closed; 'pr' for paw, ring, diamond, and closed; 'c' for claw, paw, diamond, and closed; 'cr' for claw, ring, paw, diamond, and closed; 'o' for open, ring, paw, diamond, and closed; and 'a' for including all tetramer types.

# 2 Lattice Energies

**Table S4:** Errors of the lattice energies of the X23 set, calculated with tri- and tetramer embedding methods that include additional multimer types beyond the closed type, compared to PBE0+MBD. All calculations were done with light settings on top of the PBE0+MBD-optimized structures. The mean error (ME), the mean absolute error (MAE), and the maximal error (MAX) are given in kJ/mol while the mean relative error (MRE), the mean absolute relative error (MARE), and the maximal relative error (RMAX) are given in %.

| Method | ME | MAE | MAX | MRE | MARE | RMAX |
|---|---|---|---|---|---|---|
| ME3(a3Å) | 0.6 | 1.4 | 4.0 | -0.4 | 1.6 | 6.1 |
| ME3(a4Å) | -0.3 | 0.5 | 1.5 | 0.3 | 0.6 | 1.5 |
| ME3(a5Å) | -0.4 | 0.6 | 1.6 | 0.4 | 0.7 | 2.4 |
| ME3(a6Å) | -0.7 | 1.2 | 5.8 | 1.0 | 1.3 | 5.2 |
| ME4(a3Å) | -0.5 | 1.4 | 4.7 | 0.2 | 1.5 | 6.7 |
| ME4(a4Å) | 0.5 | 0.6 | 2.3 | -0.5 | 0.7 | 2.2 |
| ME4(d4Å) | 0.1 | 0.3 | 1.1 | -0.0 | 0.4 | 1.5 |
| ME4(p4Å) | 0.0 | 0.3 | 1.7 | 0.0 | 0.4 | 2.3 |
| ME4(r4Å) | 0.0 | 0.4 | 1.2 | 0.0 | 0.4 | 1.8 |
| ME4(pr4Å) | -0.0 | 0.4 | 1.6 | 0.1 | 0.5 | 2.2 |
| ME4(c4Å) | 0.0 | 0.4 | 1.8 | 0.0 | 0.4 | 2.5 |
| ME4(cr4Å) | -0.0 | 0.4 | 1.7 | 0.1 | 0.5 | 2.4 |
| ME4(o4Å) | 0.5 | 0.6 | 2.3 | -0.5 | 0.7 | 2.0 |

**Table S5:** Errors of the lattice energies of the X23 set, calculated with tri- and tetramer embedding methods utilizing different cutoff distances for the individual multimer orders, compared to PBE0+MBD. All calculations were done with light settings on top of the PBE0+MBD-optimized structures. The mean error (ME), the mean absolute error (MAE), and the maximal error (MAX) are given in kJ/mol while the mean relative error (MRE), the mean absolute relative error (MARE), and the maximal relative error (RMAX) are given in %.

| Method | ME | MAE | MAX | MRE | MARE | RMAX |
|---|---|---|---|---|---|---|
| ME3(4/3Å) | 1.1 | 1.1 | 3.1 | -1.3 | 1.4 | 5.9 |
| ME3(5/3Å) | 1.2 | 1.2 | 3.0 | -1.4 | 1.4 | 5.8 |
| ME3(6/3Å) | 1.2 | 1.3 | 3.0 | -1.5 | 1.5 | 6.1 |
| ME3(5/4Å) | -0.2 | 0.4 | 1.2 | 0.2 | 0.4 | 1.6 |
| ME3(6/4Å) | -0.1 | 0.4 | 1.1 | 0.1 | 0.4 | 1.5 |
| ME3(7/4Å) | -0.2 | 0.3 | 1.0 | 0.1 | 0.4 | 1.4 |
| ME3(8/4Å) | -0.1 | 0.3 | 1.3 | 0.1 | 0.4 | 1.8 |
| ME3(6/5Å) | -0.5 | 0.6 | 1.3 | 0.5 | 0.7 | 1.9 |
| ME3(7/5Å) | -0.5 | 0.6 | 1.5 | 0.6 | 0.6 | 1.9 |
| ME3(8/5Å) | -0.5 | 0.5 | 1.4 | 0.5 | 0.6 | 1.6 |
| ME4(5/4/4Å) | 0.4 | 0.4 | 1.8 | -0.4 | 0.5 | 2.5 |
| ME4(6/4/4Å) | 0.4 | 0.5 | 1.7 | -0.6 | 0.6 | 2.7 |
| ME4(5/5/4Å) | -0.0 | 0.4 | 1.2 | 0.0 | 0.5 | 1.8 |
| ME4(6/5/4Å) | 0.1 | 0.4 | 1.1 | -0.1 | 0.5 | 2.4 |
| ME4(6/6/4Å) | -0.2 | 0.4 | 1.5 | 0.3 | 0.5 | 1.6 |
| ME4(6/5/5Å) | 0.3 | 0.4 | 1.2 | -0.3 | 0.5 | 2.5 |
| ME4(6/6/5Å) | -0.0 | 0.3 | 1.2 | 0.0 | 0.4 | 1.7 |

**Table S6:** Errors of the lattice energies of the X23 set, calculated with embedding methods that employ energy-based cutoffs for multimer selection, compared to PBE0+MBD. All calculations were done with light settings on top of the PBE0+MBD-optimized structures. The mean error (ME), the mean absolute error (MAE), and the maximal error (MAX) are given in kJ/mol while the mean relative error (MRE), the mean absolute relative error (MARE), and the maximal relative error (RMAX) are given in %.

| | | | | | | | % of Tri-/Tetramers saved | | |
|---|---|---|---|---|---|---|---|---|---|
| Method | ME | MAE | MAX | MRE | MARE | RMAX | Min | Avg | Max |
| ME3(4Å $>$ 0.01 kJ/mol) | -0.2 | 0.4 | 1.1 | 0.3 | 0.5 | 1.6 | 0.0 | 0.0 | 0.0 |
| ME3(4Å $>$ 0.02 kJ/mol) | -0.2 | 0.4 | 1.1 | 0.3 | 0.5 | 1.6 | 0.0 | 0.9 | 14.3 |
| ME3(4Å $>$ 0.05 kJ/mol) | -0.2 | 0.4 | 1.1 | 0.2 | 0.5 | 1.6 | 0.0 | 2.5 | 16.7 |
| ME3(4Å $>$ 0.1 kJ/mol) | -0.1 | 0.4 | 1.1 | 0.2 | 0.5 | 1.6 | 0.0 | 4.7 | 21.4 |
| ME3(4Å $>$ 0.2 kJ/mol) | -0.0 | 0.4 | 1.1 | 0.0 | 0.4 | 1.6 | 0.0 | 10.0 | 37.5 |
| ME3(4Å $>$ 0.5 kJ/mol) | 0.3 | 0.5 | 1.8 | -0.4 | 0.6 | 2.5 | 0.0 | 25.6 | 75.0 |
| ME3(4Å $>$ 1 kJ/mol) | 1.2 | 1.2 | 2.6 | -1.6 | 1.6 | 5.9 | 0.0 | 51.0 | 100.0 |
| ME3(4Å $>$ 2 kJ/mol) | 2.4 | 2.4 | 4.2 | -2.9 | 2.9 | 5.9 | 37.5 | 82.3 | 100.0 |
| ME3(4Å $>$ 5 kJ/mol) | 3.4 | 3.4 | 5.8 | -3.9 | 3.9 | 8.3 | 85.7 | 98.6 | 100.0 |
| ME3(4Å $>$ 10 kJ/mol) | 3.4 | 3.4 | 5.8 | -3.9 | 3.9 | 8.3 | 100.0 | 100.0 | 100.0 |
| ME4(5Å $>$ 0.01 kJ/mol) | 0.2 | 0.3 | 1.2 | -0.2 | 0.4 | 1.7 | 0.0 | 8.2 | 28.6 |
| ME4(5Å $>$ 0.02 kJ/mol) | 0.1 | 0.3 | 1.2 | -0.2 | 0.4 | 1.7 | 0.0 | 13.0 | 40.0 |
| ME4(5Å $>$ 0.05 kJ/mol) | 0.1 | 0.3 | 1.2 | -0.1 | 0.4 | 1.8 | 0.0 | 25.1 | 60.0 |
| ME4(5Å $>$ 0.1 kJ/mol) | 0.0 | 0.3 | 1.2 | -0.0 | 0.4 | 1.8 | 0.0 | 43.3 | 76.7 |
| ME4(5Å $>$ 0.2 kJ/mol) | -0.1 | 0.3 | 1.2 | 0.1 | 0.4 | 2.1 | 0.0 | 65.8 | 100.0 |
| ME4(5Å $>$ 0.5 kJ/mol) | -0.4 | 0.6 | 1.3 | 0.5 | 0.7 | 2.1 | 72.2 | 95.2 | 100.0 |
| ME4(5Å $>$ 1 kJ/mol) | -0.5 | 0.6 | 1.5 | 0.6 | 0.7 | 2.1 | 94.4 | 99.4 | 100.0 |
| ME4(5Å $>$ 2 kJ/mol) | -0.5 | 0.6 | 1.5 | 0.6 | 0.7 | 2.1 | 95.5 | 99.8 | 100.0 |
| ME4(5Å $>$ 5 kJ/mol) | -0.6 | 0.6 | 1.5 | 0.7 | 0.7 | 2.1 | 100.0 | 100.0 | 100.0 |
| ME4(5Å $>$ 10 kJ/mol) | -0.6 | 0.6 | 1.5 | 0.7 | 0.7 | 2.1 | 100.0 | 100.0 | 100.0 |

**Table S7:** Lattice energies in kJ/mol calculated for the respective method with light species default settings on top of PBE0+MBD/light-optimized structures (part 1).

| System | PBE0+MBD | PBE+MBD | ME1 | ME2(4Å) | ME3(4Å) | ME4(3Å) | ME4(4Å) | ME4(5Å) | ME4(6Å) |
|---|---|---|---|---|---|---|---|---|---|
| 1,4-Cyclohexanedione | -99.6 | -92.7 | -95.0 | -95.6 | -100.0 | -99.4 | -99.2 | -99.3 | -99.3 |
| Acetic acid | -80.1 | -77.3 | -78.0 | -77.4 | -80.6 | -78.4 | -80.0 | -80.3 | -80.2 |
| Adamantane | -81.3 | -76.7 | -79.6 | -77.6 | -81.5 | -81.2 | -81.2 | -81.2 | -81.2 |
| Ammonia | -42.7 | -45.3 | -45.2 | -39.2 | -42.9 | -42.5 | -42.0 | -42.1 | -42.7 |
| Anthracene | -124.5 | -111.1 | -114.8 | -121.3 | -124.3 | -124.0 | -124.0 | -124.1 | -124.1 |
| Benzene | -60.4 | -56.2 | -57.4 | -57.8 | -60.2 | -60.0 | -60.0 | -60.2 | -60.3 |
| Carbon dioxide | -28.0 | -24.6 | -27.7 | -26.3 | -28.2 | -27.7 | -28.1 | -28.3 | -28.0 |
| Cyanamide | -90.5 | -92.1 | -92.9 | -87.0 | -91.5 | -90.0 | -90.7 | -90.8 | -89.5 |
| Cytosine | -171.5 | -164.5 | -164.6 | -167.3 | -171.7 | -167.2 | -171.1 | -171.6 | -172.3 |
| Ethyl carbamate | -95.1 | -91.1 | -93.4 | -91.7 | -95.6 | -95.0 | -95.1 | -94.9 | -94.9 |
| Formamide | -85.9 | -84.8 | -83.6 | -83.0 | -87.1 | -85.3 | -86.4 | -86.1 | -85.8 |
| Hexamine | -95.8 | -89.8 | -91.5 | -94.1 | -96.0 | -95.5 | -95.5 | -95.5 | -96.0 |
| Imidazole | -98.3 | -96.1 | -96.5 | -95.9 | -99.0 | -96.8 | -98.7 | -98.6 | -98.3 |
| Naphthalene | -91.6 | -82.8 | -85.2 | -88.5 | -91.5 | -91.2 | -91.2 | -91.3 | -91.3 |
| Oxalic acid $\alpha$ | -107.4 | -98.1 | -102.7 | -104.0 | -107.2 | -106.8 | -106.0 | -107.0 | -107.0 |
| Oxalic acid $\beta$ | -107.6 | -100.3 | -103.4 | -102.5 | -107.6 | -105.8 | -106.8 | -107.3 | -107.5 |
| Pyrazine | -69.6 | -66.1 | -67.6 | -66.7 | -70.0 | -66.9 | -69.4 | -69.4 | -69.5 |
| Pyrazole | -87.5 | -85.0 | -85.6 | -84.9 | -87.4 | -86.8 | -87.1 | -87.3 | -87.4 |
| s-Triazine | -64.0 | -58.7 | -60.7 | -60.4 | -64.5 | -61.1 | -63.8 | -63.8 | -63.9 |
| s-Trioxane | -71.0 | -64.9 | -66.6 | -66.8 | -69.9 | -69.3 | -69.3 | -69.7 | -69.7 |
| Succinic acid | -142.2 | -136.5 | -137.2 | -136.5 | -142.9 | -140.6 | -141.8 | -142.1 | -142.0 |
| Uracil | -147.2 | -139.8 | -140.3 | -143.3 | -147.8 | -143.9 | -147.1 | -147.1 | -147.2 |
| Urea | -112.5 | -109.9 | -110.2 | -109.1 | -113.1 | -113.0 | -112.7 | -112.7 | -111.3 |

**Table S8:** Lattice energies in kJ/mol calculated for the respective method with light species default settings on top of PBE0+MBD/light-optimized structures (part 2).

| System | ME3(a3Å) | ME3(a4Å) | ME3(a5Å) | ME3(a6Å) |
|---|---|---|---|---|
| 1,4-Cyclohexanedione | -98.0 | -100.3 | -100.4 | -100.0 |
| Acetic acid | -79.6 | -81.0 | -81.0 | -80.7 |
| Adamantane | -81.2 | -81.2 | -81.7 | -81.7 |
| Ammonia | -42.2 | -43.1 | -41.7 | -44.9 |
| Anthracene | -124.8 | -125.2 | -125.4 | -124.8 |
| Benzene | -60.9 | -60.9 | -61.0 | -61.1 |
| Carbon dioxide | -27.7 | -28.2 | -28.0 | -28.1 |
| Cyanamide | -88.7 | -90.7 | -90.9 | -91.3 |
| Cytosine | -168.8 | -172.4 | -170.3 | -167.0 |
| Ethyl carbamate | -94.3 | -94.9 | -95.7 | -96.4 |
| Formamide | -82.5 | -85.7 | -86.1 | -88.6 |
| Hexamine | -95.5 | -95.5 | -95.5 | -96.2 |
| Imidazole | -97.5 | -97.8 | -97.9 | -99.1 |
| Naphthalene | -91.8 | -92.2 | -92.3 | -91.6 |
| Oxalic acid $\alpha$ | -108.1 | -107.8 | -107.9 | -107.6 |
| Oxalic acid $\beta$ | -107.4 | -108.8 | -108.9 | -108.9 |
| Pyrazine | -73.5 | -70.1 | -70.1 | -70.3 |
| Pyrazole | -87.1 | -87.8 | -87.6 | -88.2 |
| s-Triazine | -68.0 | -64.6 | -65.0 | -64.6 |
| s-Trioxane | -69.9 | -69.9 | -71.6 | -71.4 |
| Succinic acid | -139.6 | -143.7 | -143.9 | -144.2 |
| Uracil | -145.7 | -147.6 | -147.9 | -145.6 |
| Urea | -108.6 | -112.5 | -112.5 | -118.3 |

**Table S9:** Lattice energies in kJ/mol calculated for the respective method with light species default settings on top of PBE0+MBD/light-optimized structures (part 3).

| System | ME4(a3Å) | ME4(a4Å) | ME4(d4Å) | ME4(p4Å) | ME4(r4Å) | ME4(pr4Å) | ME4(c4Å) | ME4(cr4Å) | ME4(o4Å) |
|---|---|---|---|---|---|---|---|---|---|
| 1,4-Cyclohexanedione | -101.0 | -99.0 | -99.1 | -98.9 | -99.0 | -98.8 | -98.9 | -98.7 | -99.0 |
| Acetic acid | -80.8 | -80.1 | -80.2 | -80.3 | -80.1 | -80.3 | -80.3 | -80.2 | -80.1 |
| Adamantane | -81.6 | -81.6 | -81.3 | -81.4 | -81.5 | -81.6 | -81.4 | -81.6 | -81.6 |
| Ammonia | -43.3 | -41.9 | -43.3 | -42.9 | -43.5 | -43.1 | -43.0 | -43.2 | -41.9 |
| Anthracene | -124.6 | -124.5 | -124.4 | -124.2 | -124.3 | -124.2 | -124.2 | -124.1 | -124.5 |
| Benzene | -60.5 | -60.5 | -60.5 | -60.3 | -60.6 | -60.5 | -60.3 | -60.5 | -60.5 |
| Carbon dioxide | -27.7 | -27.8 | -27.9 | -28.1 | -27.9 | -28.1 | -28.1 | -28.1 | -27.8 |
| Cyanamide | -90.8 | -90.3 | -90.0 | -90.9 | -90.1 | -90.9 | -91.0 | -91.1 | -90.2 |
| Cytosine | -175.2 | -169.1 | -170.6 | -171.0 | -170.2 | -170.7 | -171.0 | -170.7 | -169.1 |
| Ethyl carbamate | -96.1 | -95.4 | -95.7 | -95.7 | -96.0 | -96.0 | -95.7 | -96.0 | -95.4 |
| Formamide | -88.3 | -85.1 | -86.6 | -86.8 | -86.9 | -87.1 | -86.8 | -87.1 | -85.1 |
| Hexamine | -96.4 | -96.4 | -96.2 | -96.3 | -96.3 | -96.4 | -96.3 | -96.3 | -96.4 |
| Imidazole | -99.7 | -98.1 | -98.1 | -98.5 | -98.2 | -98.5 | -98.4 | -98.5 | -98.1 |
| Naphthalene | -91.6 | -91.4 | -91.5 | -91.4 | -91.5 | -91.4 | -91.4 | -91.3 | -91.5 |
| Oxalic acid $\alpha$ | -106.2 | -106.6 | -107.3 | -107.3 | -107.3 | -107.4 | -107.4 | -107.4 | -106.6 |
| Oxalic acid $\beta$ | -108.2 | -107.3 | -107.9 | -107.9 | -108.0 | -108.0 | -108.0 | -108.1 | -107.2 |
| Pyrazine | -64.9 | -70.0 | -69.7 | -69.7 | -69.7 | -69.8 | -69.7 | -69.8 | -70.0 |
| Pyrazole | -87.5 | -87.1 | -87.5 | -87.5 | -87.5 | -87.5 | -87.5 | -87.5 | -87.1 |
| s-Triazine | -61.8 | -63.9 | -64.0 | -64.1 | -64.1 | -64.1 | -64.1 | -64.1 | -63.9 |
| s-Trioxane | -69.5 | -69.5 | -69.9 | -69.3 | -70.0 | -69.4 | -69.2 | -69.3 | -69.6 |
| Succinic acid | -145.2 | -142.3 | -142.3 | -142.3 | -142.4 | -142.3 | -142.3 | -142.3 | -142.3 |
| Uracil | -148.7 | -145.2 | -146.6 | -146.7 | -146.7 | -146.8 | -146.7 | -146.8 | -145.2 |
| Urea | -116.3 | -110.6 | -111.8 | -112.2 | -112.1 | -112.5 | -112.3 | -112.5 | -110.6 |

**Table S10:** Lattice energies in kJ/mol calculated for the respective method with light species default settings on top of PBE0+MBD/light-optimized structures (part 4).

| System | ME3(4/3Å) | ME3(5/3Å) | ME3(6/3Å) | ME3(5/4Å) | ME3(6/4Å) | ME3(7/4Å) | ME3(8/4Å) | ME3(6/5Å) | ME3(7/5Å) | ME3(8/5Å) |
|---|---|---|---|---|---|---|---|---|---|---|
| 1,4-Cyclohexanedione | -98.6 | -98.7 | -98.8 | -100.0 | -100.1 | -100.1 | -100.1 | -100.2 | -100.1 | -100.1 |
| Acetic acid | -78.4 | -78.5 | -78.5 | -80.7 | -80.8 | -80.8 | -80.7 | -81.1 | -81.1 | -81.0 |
| Adamantane | -81.5 | -81.3 | -81.3 | -81.3 | -81.3 | -81.3 | -81.3 | -81.8 | -81.8 | -81.8 |
| Ammonia | -42.4 | -42.4 | -41.9 | -42.9 | -42.5 | -42.6 | -42.6 | -42.7 | -42.8 | -42.8 |
| Anthracene | -124.0 | -124.0 | -124.2 | -124.3 | -124.5 | -124.5 | -124.5 | -124.6 | -124.6 | -124.6 |
| Benzene | -60.2 | -60.2 | -60.2 | -60.2 | -60.2 | -60.2 | -60.3 | -60.7 | -60.7 | -60.8 |
| Carbon dioxide | -26.3 | -26.3 | -26.3 | -28.2 | -28.1 | -28.1 | -28.1 | -28.5 | -28.5 | -28.4 |
| Cyanamide | -89.2 | -89.1 | -88.9 | -91.4 | -91.2 | -91.2 | -91.1 | -91.7 | -91.7 | -91.6 |
| Cytosine | -168.8 | -169.2 | -169.5 | -172.2 | -172.4 | -172.0 | -171.2 | -172.7 | -172.2 | -171.5 |
| Ethyl carbamate | -95.1 | -94.7 | -94.6 | -95.2 | -95.1 | -95.1 | -95.2 | -95.6 | -95.7 | -95.7 |
| Formamide | -84.5 | -83.8 | -83.4 | -86.3 | -85.9 | -86.0 | -86.0 | -87.1 | -87.1 | -87.1 |
| Hexamine | -96.0 | -96.0 | -95.7 | -96.0 | -95.7 | -95.7 | -95.7 | -95.7 | -95.7 | -95.7 |
| Imidazole | -96.9 | -96.8 | -96.4 | -98.9 | -98.5 | -98.5 | -98.5 | -98.6 | -98.6 | -98.6 |
| Naphthalene | -91.2 | -91.2 | -91.4 | -91.5 | -91.6 | -91.6 | -91.6 | -91.8 | -91.7 | -91.7 |
| Oxalic acid $\alpha$ | -107.4 | -107.3 | -107.3 | -107.2 | -107.2 | -107.2 | -107.1 | -107.9 | -107.9 | -107.9 |
| Oxalic acid $\beta$ | -105.5 | -105.5 | -105.5 | -107.6 | -107.5 | -107.6 | -107.5 | -108.6 | -108.6 | -108.5 |
| Pyrazine | -68.2 | -68.2 | -68.1 | -70.0 | -69.9 | -69.9 | -69.9 | -69.9 | -69.9 | -69.9 |
| Pyrazole | -86.8 | -86.8 | -86.7 | -87.4 | -87.3 | -87.3 | -87.3 | -87.7 | -87.7 | -87.8 |
| s-Triazine | -62.5 | -62.3 | -62.4 | -64.3 | -64.4 | -64.4 | -64.4 | -64.7 | -64.7 | -64.7 |
| s-Trioxane | -69.9 | -69.8 | -69.9 | -69.8 | -69.9 | -70.0 | -69.7 | -70.5 | -70.6 | -70.3 |
| Succinic acid | -139.1 | -139.3 | -139.3 | -143.0 | -143.0 | -143.1 | -143.1 | -143.6 | -143.7 | -143.7 |
| Uracil | -144.9 | -144.9 | -145.1 | -147.7 | -147.9 | -147.9 | -147.9 | -148.0 | -148.0 | -148.0 |
| Urea | -111.5 | -111.5 | -110.2 | -113.1 | -111.8 | -112.9 | -113.1 | -111.8 | -112.9 | -113.1 |

**Table S11:** Lattice energies in kJ/mol calculated for the respective method with light species default settings on top of PBE0+MBD/light-optimized structures (part 5).

| System | ME4(5/4/4Å) | ME4(6/4/4Å) | ME4(5/5/4Å) | ME4(6/5/4Å) | ME4(6/6/4Å) | ME4(6/5/5Å) | ME4(6/6/5Å) |
|---|---|---|---|---|---|---|---|
| 1,4-Cyclohexanedione | -99.2 | -99.3 | -99.3 | -99.4 | -99.4 | -99.4 | -99.4 |
| Acetic acid | -80.1 | -80.2 | -80.5 | -80.5 | -80.5 | -80.3 | -80.3 |
| Adamantane | -81.0 | -81.0 | -81.5 | -81.5 | -81.5 | -81.2 | -81.2 |
| Ammonia | -42.0 | -41.5 | -42.1 | -41.7 | -43.0 | -41.7 | -43.0 |
| Anthracene | -124.0 | -124.3 | -124.1 | -124.4 | -124.7 | -124.4 | -124.7 |
| Benzene | -60.0 | -60.0 | -60.5 | -60.5 | -60.8 | -60.2 | -60.5 |
| Carbon dioxide | -28.1 | -28.0 | -28.5 | -28.4 | -28.4 | -28.3 | -28.3 |
| Cyanamide | -90.6 | -90.4 | -91.1 | -90.9 | -90.6 | -90.6 | -90.3 |
| Cytosine | -171.6 | -171.9 | -171.8 | -172.1 | -172.9 | -171.9 | -172.7 |
| Ethyl carbamate | -94.8 | -94.6 | -95.3 | -95.2 | -95.4 | -94.7 | -95.0 |
| Formamide | -85.7 | -85.3 | -86.8 | -86.4 | -87.0 | -85.7 | -86.2 |
| Hexamine | -95.5 | -95.3 | -95.5 | -95.3 | -95.6 | -95.3 | -95.6 |
| Imidazole | -98.6 | -98.2 | -98.7 | -98.3 | -98.8 | -98.3 | -98.7 |
| Naphthalene | -91.2 | -91.4 | -91.3 | -91.5 | -91.9 | -91.5 | -91.9 |
| Oxalic acid $\alpha$ | -106.0 | -106.0 | -106.7 | -106.7 | -106.8 | -107.0 | -107.1 |
| Oxalic acid $\beta$ | -106.9 | -106.8 | -107.9 | -107.8 | -108.3 | -107.2 | -107.7 |
| Pyrazine | -69.4 | -69.3 | -69.4 | -69.3 | -69.8 | -69.3 | -69.8 |
| Pyrazole | -87.1 | -87.0 | -87.5 | -87.4 | -87.7 | -87.2 | -87.4 |
| s-Triazine | -63.7 | -63.7 | -64.0 | -64.1 | -64.1 | -63.9 | -63.9 |
| s-Trioxane | -69.2 | -69.3 | -69.8 | -69.9 | -69.9 | -69.8 | -69.8 |
| Succinic acid | -142.0 | -142.0 | -142.5 | -142.5 | -142.5 | -142.1 | -142.0 |
| Uracil | -147.1 | -147.3 | -147.2 | -147.4 | -147.6 | -147.3 | -147.5 |
| Urea | -112.7 | -111.4 | -112.7 | -111.4 | -112.0 | -111.4 | -112.0 |

**Table S12:** Lattice energies in kJ/mol calculated for the respective method with light species default settings on top of PBE0+MBD/light-optimized structures (part 6).

| | ME3(4Å $> x$ kJ/mol) | | | | | | | | | |
|---|---|---|---|---|---|---|---|---|---|---|
| System | $x = 0.01$ | $x = 0.02$ | $x = 0.05$ | $x = 0.1$ | $x = 0.2$ | $x = 0.5$ | $x = 1$ | $x = 2$ | $x = 5$ | $x = 10$ |
| 1,4-Cyclohexanedione | -100.0 | -99.9 | -99.9 | -99.5 | -99.5 | -99.3 | -98.7 | -97.5 | -95.6 | -95.6 |
| Acetic acid | -80.6 | -80.6 | -80.3 | -80.1 | -79.9 | -79.1 | -78.4 | -78.4 | -77.4 | -77.4 |
| Adamantane | -81.5 | -81.5 | -81.5 | -81.5 | -81.5 | -81.5 | -81.5 | -77.6 | -77.6 | -77.6 |
| Ammonia | -42.9 | -42.9 | -42.9 | -42.9 | -42.8 | -42.4 | -41.0 | -41.0 | -39.2 | -39.2 |
| Anthracene | -124.3 | -124.3 | -124.3 | -124.3 | -124.2 | -124.0 | -123.6 | -122.4 | -121.3 | -121.3 |
| Benzene | -60.2 | -60.2 | -60.2 | -60.2 | -60.2 | -60.2 | -58.4 | -57.8 | -57.8 | -57.8 |
| Carbon dioxide | -28.2 | -28.2 | -28.2 | -28.2 | -28.2 | -27.9 | -26.3 | -26.3 | -26.3 | -26.3 |
| Cyanamide | -91.5 | -91.5 | -91.5 | -91.5 | -91.3 | -91.0 | -91.0 | -89.9 | -87.0 | -87.0 |
| Cytosine | -171.7 | -171.7 | -171.7 | -171.7 | -171.7 | -170.0 | -169.8 | -169.4 | -167.3 | -167.3 |
| Ethyl carbamate | -95.6 | -95.6 | -95.6 | -95.6 | -95.6 | -95.3 | -94.2 | -91.7 | -91.7 | -91.7 |
| Formamide | -87.1 | -87.1 | -87.1 | -87.1 | -85.5 | -85.2 | -85.2 | -84.3 | -83.0 | -83.0 |
| Hexamine | -96.0 | -96.0 | -96.0 | -96.0 | -96.0 | -96.0 | -94.1 | -94.1 | -94.1 | -94.1 |
| Imidazole | -99.0 | -99.0 | -98.9 | -98.7 | -98.7 | -98.2 | -97.7 | -96.6 | -95.9 | -95.9 |
| Naphthalene | -91.5 | -91.5 | -91.5 | -91.5 | -91.4 | -91.2 | -90.2 | -88.5 | -88.5 | -88.5 |
| Oxalic acid $\alpha$ | -107.2 | -107.2 | -107.2 | -107.2 | -107.2 | -107.0 | -106.9 | -106.0 | -103.5 | -104.0 |
| Oxalic acid $\beta$ | -107.6 | -107.6 | -107.0 | -107.0 | -107.0 | -107.0 | -105.5 | -104.1 | -102.5 | -102.5 |
| Pyrazine | -70.0 | -70.0 | -70.0 | -70.0 | -70.0 | -70.0 | -67.4 | -66.7 | -66.7 | -66.7 |
| Pyrazole | -87.4 | -87.4 | -87.4 | -87.3 | -87.3 | -87.0 | -86.1 | -85.2 | -84.9 | -84.9 |
| s-Triazine | -64.5 | -64.5 | -64.5 | -64.5 | -64.5 | -63.5 | -63.5 | -60.4 | -60.4 | -60.4 |
| s-Trioxane | -69.9 | -69.9 | -69.9 | -69.9 | -69.9 | -69.2 | -68.4 | -66.8 | -66.8 | -66.8 |
| Succinic acid | -142.9 | -142.9 | -142.9 | -142.9 | -142.9 | -142.9 | -140.6 | -138.1 | -136.5 | -136.5 |
| Uracil | -147.8 | -147.8 | -147.5 | -147.5 | -147.5 | -147.4 | -146.9 | -145.6 | -143.3 | -143.3 |
| Urea | -113.1 | -113.0 | -113.0 | -113.0 | -113.0 | -112.5 | -112.5 | -111.5 | -109.1 | -109.1 |

**Table S13:** Lattice energies in kJ/mol calculated for the respective method with light species default settings on top of PBE0+MBD/light-optimized structures (part 7).

| | ME4(5Å > $x$ kJ/mol) | | | | | | | | | |
|---|---|---|---|---|---|---|---|---|---|---|
| System | $x = 0.01$ | $x = 0.02$ | $x = 0.05$ | $x = 0.1$ | $x = 0.2$ | $x = 0.5$ | $x = 1$ | $x = 2$ | $x = 5$ | $x = 10$ |
| 1,4-Cyclohexanedione | -99.3 | -99.3 | -99.3 | -99.3 | -99.4 | -99.9 | -100.0 | -100.0 | -100.0 | -100.0 |
| Acetic acid | -80.3 | -80.4 | -80.5 | -80.6 | -81.0 | -81.1 | -81.1 | -81.1 | -81.1 | -81.1 |
| Adamantane | -81.2 | -81.2 | -81.2 | -81.2 | -81.4 | -81.8 | -81.8 | -81.8 | -81.8 | -81.8 |
| Ammonia | -42.1 | -42.2 | -42.1 | -42.2 | -42.7 | -42.9 | -43.1 | -43.1 | -43.1 | -43.1 |
| Anthracene | -124.1 | -124.1 | -124.1 | -124.2 | -124.2 | -124.4 | -124.4 | -124.4 | -124.4 | -124.4 |
| Benzene | -60.2 | -60.2 | -60.3 | -60.4 | -60.5 | -60.7 | -60.7 | -60.7 | -60.7 | -60.7 |
| Carbon dioxide | -28.3 | -28.3 | -28.5 | -28.5 | -28.6 | -28.6 | -28.6 | -28.6 | -28.6 | -28.6 |
| Cyanamide | -90.8 | -90.8 | -90.9 | -90.9 | -91.1 | -91.2 | -91.8 | -91.9 | -91.9 | -91.9 |
| Cytosine | -171.6 | -171.6 | -171.6 | -171.5 | -171.7 | -172.3 | -172.4 | -172.4 | -172.4 | -172.4 |
| Ethyl carbamate | -94.9 | -94.9 | -94.9 | -95.1 | -95.2 | -95.6 | -95.6 | -95.7 | -95.7 | -95.7 |
| Formamide | -86.1 | -86.2 | -86.2 | -86.3 | -86.5 | -87.1 | -87.4 | -87.4 | -87.4 | -87.4 |
| Hexamine | -95.5 | -95.5 | -95.5 | -95.5 | -95.5 | -96.0 | -96.0 | -96.0 | -96.0 | -96.0 |
| Imidazole | -98.6 | -98.6 | -98.7 | -98.8 | -98.9 | -99.0 | -99.0 | -99.0 | -99.0 | -99.0 |
| Naphthalene | -91.3 | -91.3 | -91.3 | -91.4 | -91.4 | -91.6 | -91.6 | -91.6 | -91.6 | -91.6 |
| Oxalic acid $\alpha$ | -106.9 | -106.9 | -106.9 | -107.0 | -106.9 | -106.5 | -107.4 | -107.4 | -107.9 | -107.9 |
| Oxalic acid $\beta$ | -107.3 | -107.3 | -107.3 | -107.5 | -107.9 | -108.3 | -108.6 | -108.6 | -108.6 | -108.6 |
| Pyrazine | -69.4 | -69.4 | -69.4 | -69.4 | -69.4 | -70.0 | -70.0 | -70.0 | -70.0 | -70.0 |
| Pyrazole | -87.3 | -87.3 | -87.3 | -87.5 | -87.6 | -87.8 | -87.8 | -87.8 | -87.8 | -87.8 |
| s-Triazine | -63.9 | -63.9 | -63.9 | -64.0 | -64.0 | -64.7 | -64.7 | -64.7 | -64.7 | -64.7 |
| s-Trioxane | -69.8 | -69.8 | -69.8 | -69.8 | -69.8 | -70.4 | -70.4 | -70.4 | -70.4 | -70.4 |
| Succinic acid | -142.1 | -142.2 | -142.4 | -142.5 | -142.5 | -143.6 | -143.6 | -143.6 | -143.6 | -143.6 |
| Uracil | -147.1 | -147.1 | -147.2 | -147.3 | -147.5 | -147.8 | -147.8 | -147.8 | -147.8 | -147.8 |
| Urea | -112.7 | -112.7 | -112.9 | -112.9 | -113.0 | -113.1 | -113.1 | -113.1 | -113.1 | -113.1 |

# 3 Unit-Cell Volumes

**Table S14:** Unit-cell volumes in Å$^3$ calculated for the respective method with light species default settings.

| System | PBE0+MBD | PBE+MBD | ME1 | ME2(4Å) | ME3(3Å) | ME3(4Å) | ME3(5Å) |
|---|---|---|---|---|---|---|---|
| 1,4-Cyclohexanedione | 271.3 | 280.7 | 278.3 | 275.8 | 271.8 | 270.6 | 270.5 |
| Acetic acid | 291.5 | 300.0 | 299.5 | 295.6 | 294.7 | 291.2 | 290.9 |
| Adamantane | 369.2 | 383.4 | 377.9 | 376.7 | 371.7 | 371.7 | 371.3 |
| Ammonia | 123.9 | 124.8 | 124.0 | 130.6 | 124.8 | 122.6 | 122.8 |
| Anthracene | 444.0 | 460.1 | 454.9 | 448.1 | 445.6 | 445.4 | 445.1 |
| Benzene | 453.2 | 469.0 | 464.1 | 461.0 | 454.6 | 454.6 | 452.7 |
| Carbon dioxide | 179.4 | 188.2 | 185.6 | 184.3 | 185.5 | 179.6 | 178.4 |
| Cyanamide | 411.4 | 422.4 | 417.1 | 430.2 | 419.5 | 410.0 | 409.2 |
| Cytosine | 457.6 | 478.8 | 474.3 | 466.1 | 474.9 | 459.1 | 456.2 |
| Ethyl carbamate | 237.2 | 245.1 | 242.2 | 240.4 | 236.8 | 236.8 | 236.6 |
| Formamide | 218.1 | 224.7 | 224.6 | 224.5 | 223.6 | 217.9 | 217.8 |
| Hexamine | 319.8 | 330.1 | 324.6 | 321.9 | 320.3 | 320.3 | 320.3 |
| Imidazole | 344.7 | 358.3 | 355.2 | 353.3 | 352.6 | 343.3 | 343.3 |
| Naphthalene | 333.7 | 346.1 | 342.1 | 337.8 | 334.5 | 334.2 | 333.9 |
| Oxalic acid $\alpha$ | 303.3 | 315.9 | 314.5 | 307.1 | 304.5 | 304.5 | 306.0 |
| Oxalic acid $\beta$ | 152.5 | 159.4 | 158.6 | 155.9 | 155.7 | 151.6 | 151.5 |
| Pyrazine | 195.5 | 201.0 | 199.2 | 198.7 | 198.2 | 194.6 | 194.6 |
| Pyrazole | 689.8 | 717.8 | 711.3 | 702.1 | 693.7 | 690.9 | 686.8 |
| s-Triazine | 549.1 | 567.2 | 563.4 | 558.7 | 557.9 | 547.5 | 549.1 |
| s-Trioxane | 591.9 | 611.5 | 606.7 | 600.3 | 591.1 | 591.1 | 589.0 |
| Succinic acid | 237.3 | 246.4 | 244.3 | 241.8 | 239.0 | 236.5 | 234.9 |
| Uracil | 445.8 | 462.7 | 459.1 | 450.7 | 454.1 | 446.1 | 445.8 |
| Urea | 141.8 | 144.1 | 143.7 | 143.4 | 142.2 | 141.5 | 141.5 |

# 4 Phonon Densities of States

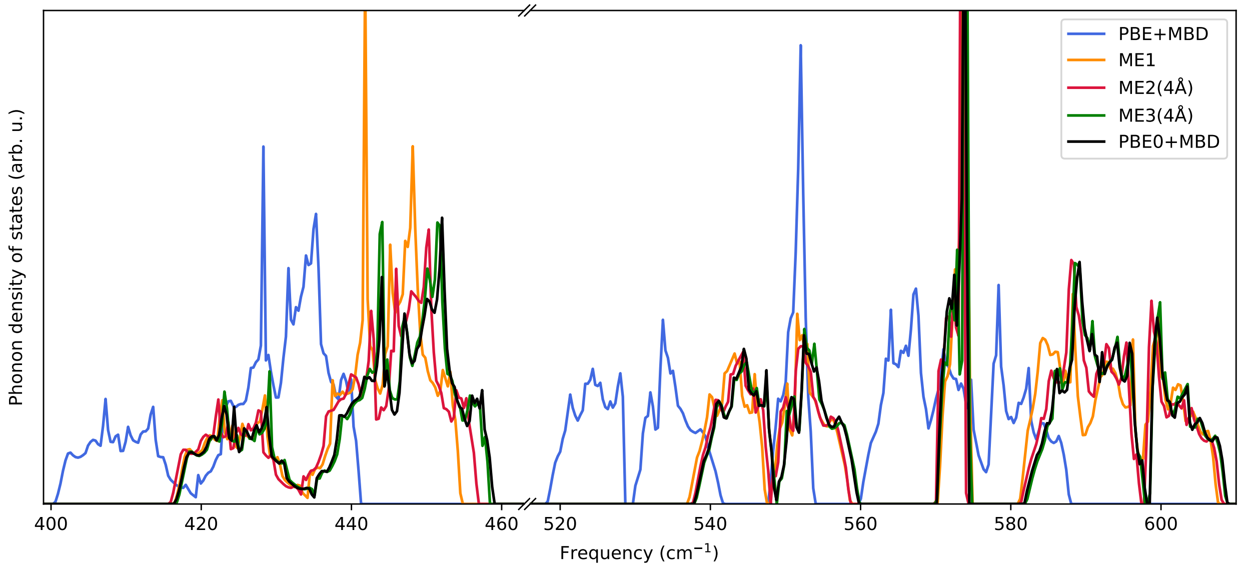


**Figure S2:** Phonon density of states of uracil between 400 and 610 cm$^{-1}$ calculated on top of optimized structures for several methods.

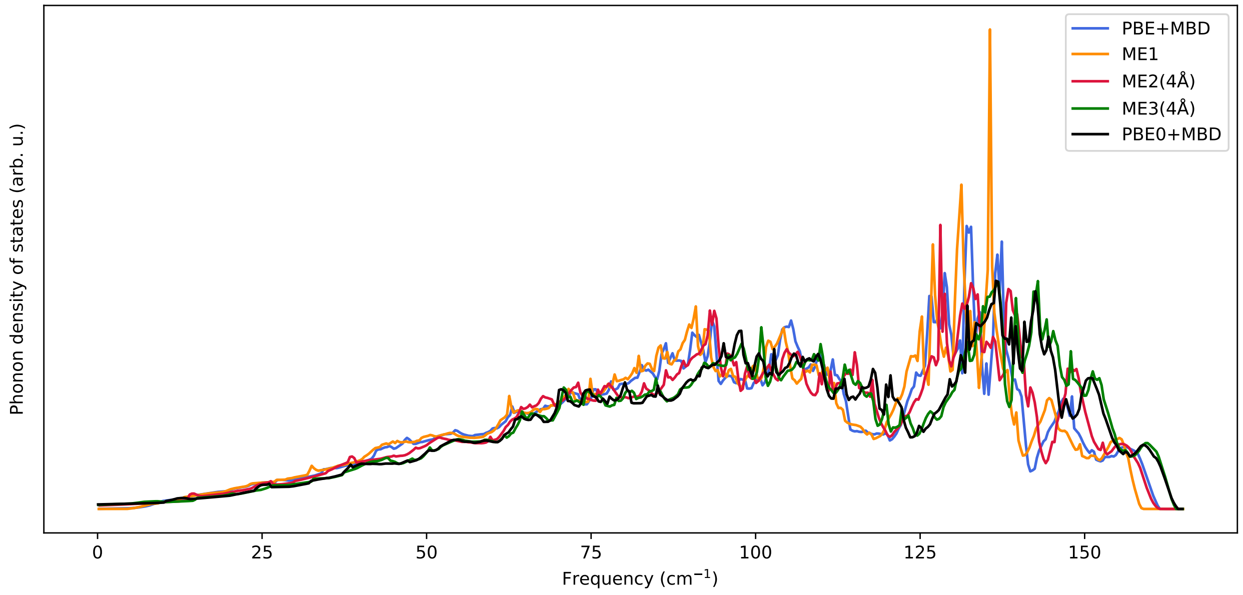


**Figure S3:** Low-frequency phonon density of states of uracil calculated on top of optimized structures for several methods.

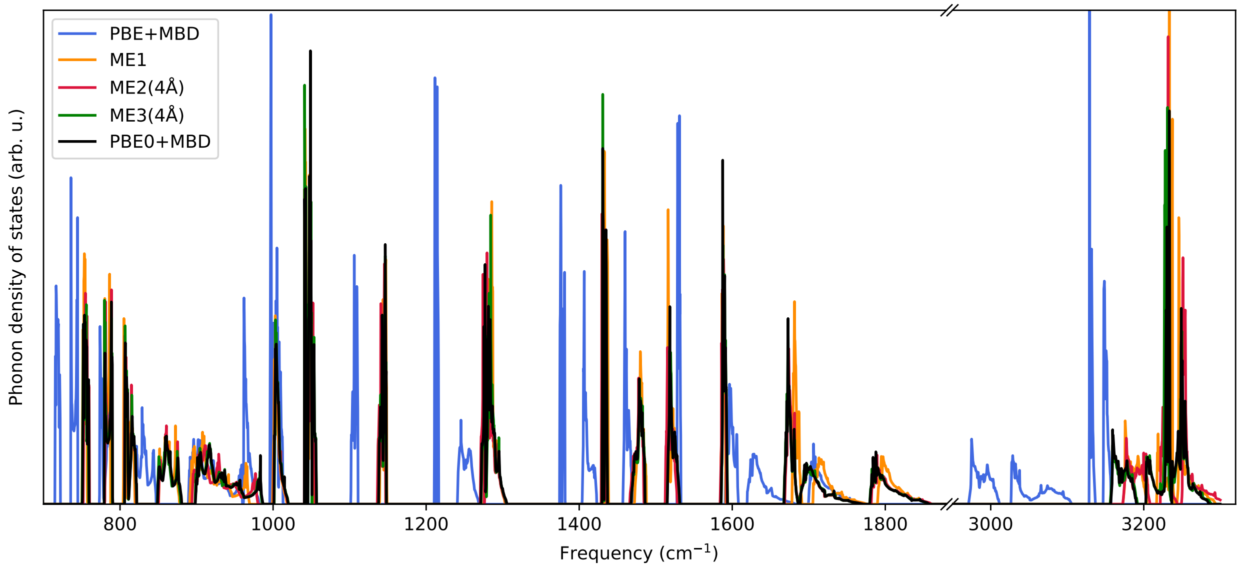


**Figure S4:** Phonon density of states of uracil above 700 $cm^{-1}$ calculated on top of optimized structures for several methods.
